# Supplementary material for: HQC-NBV: A Hybrid Quantum-Classical View Planning Approach
Source: arXiv:2505.05212 source file (2025-05-08)
Supplement: Supplementary file 1 [file X_suppl.tex]

\clearpage
\setcounter{page}{1}
\maketitlesupplementary

\section{Experimental Setup and Evaluation Metrics}
\label{sec:eval}
In the \textbf{Experiments and Results} section, we assess our approach in three different scenes. The visualized scene setup S1, S2, and S3 with initialized view are shown in Figure \ref{fig:s1,fig:s2,fig:s3}, respectively: 
\begin{figure}
    \centering
    \includegraphics[width=0.8\linewidth]{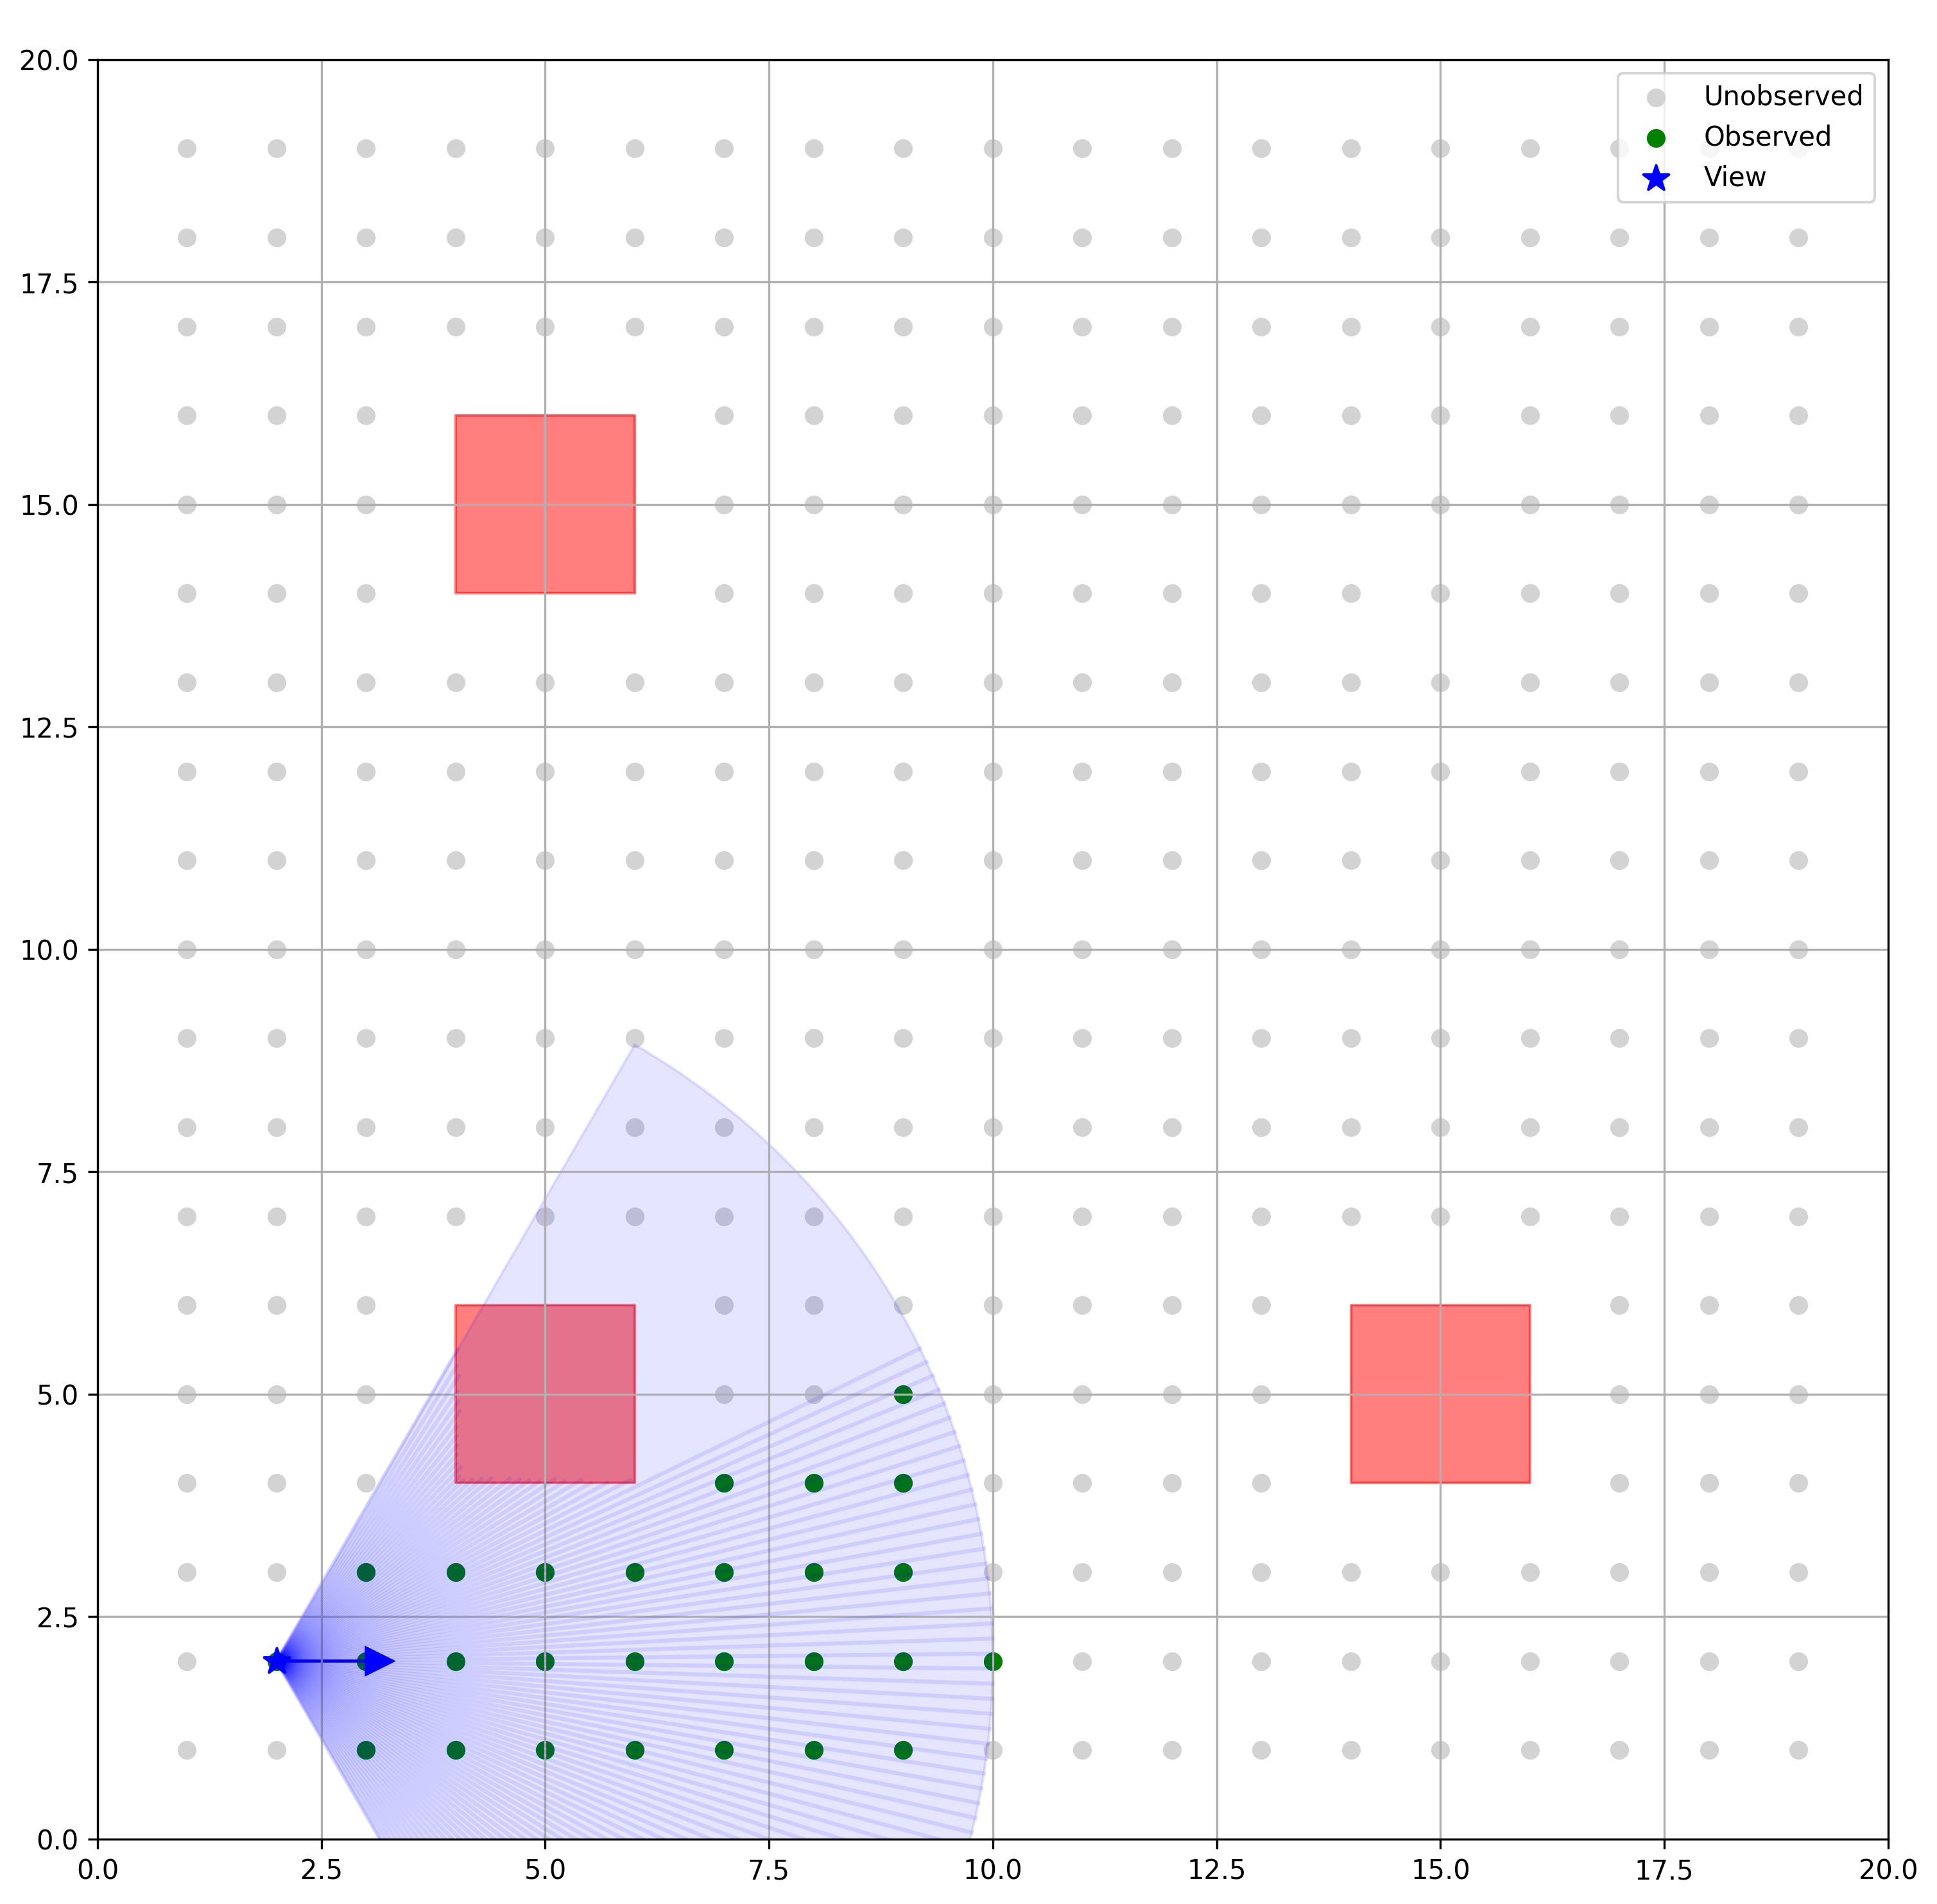}
    \caption{Scene 1: Surrounding obstacles in area $20\times20$ $\text{unit}^2$.}
    \label{fig:s1}
\end{figure}
\begin{figure}
    \centering
    \includegraphics[width=0.8\linewidth]{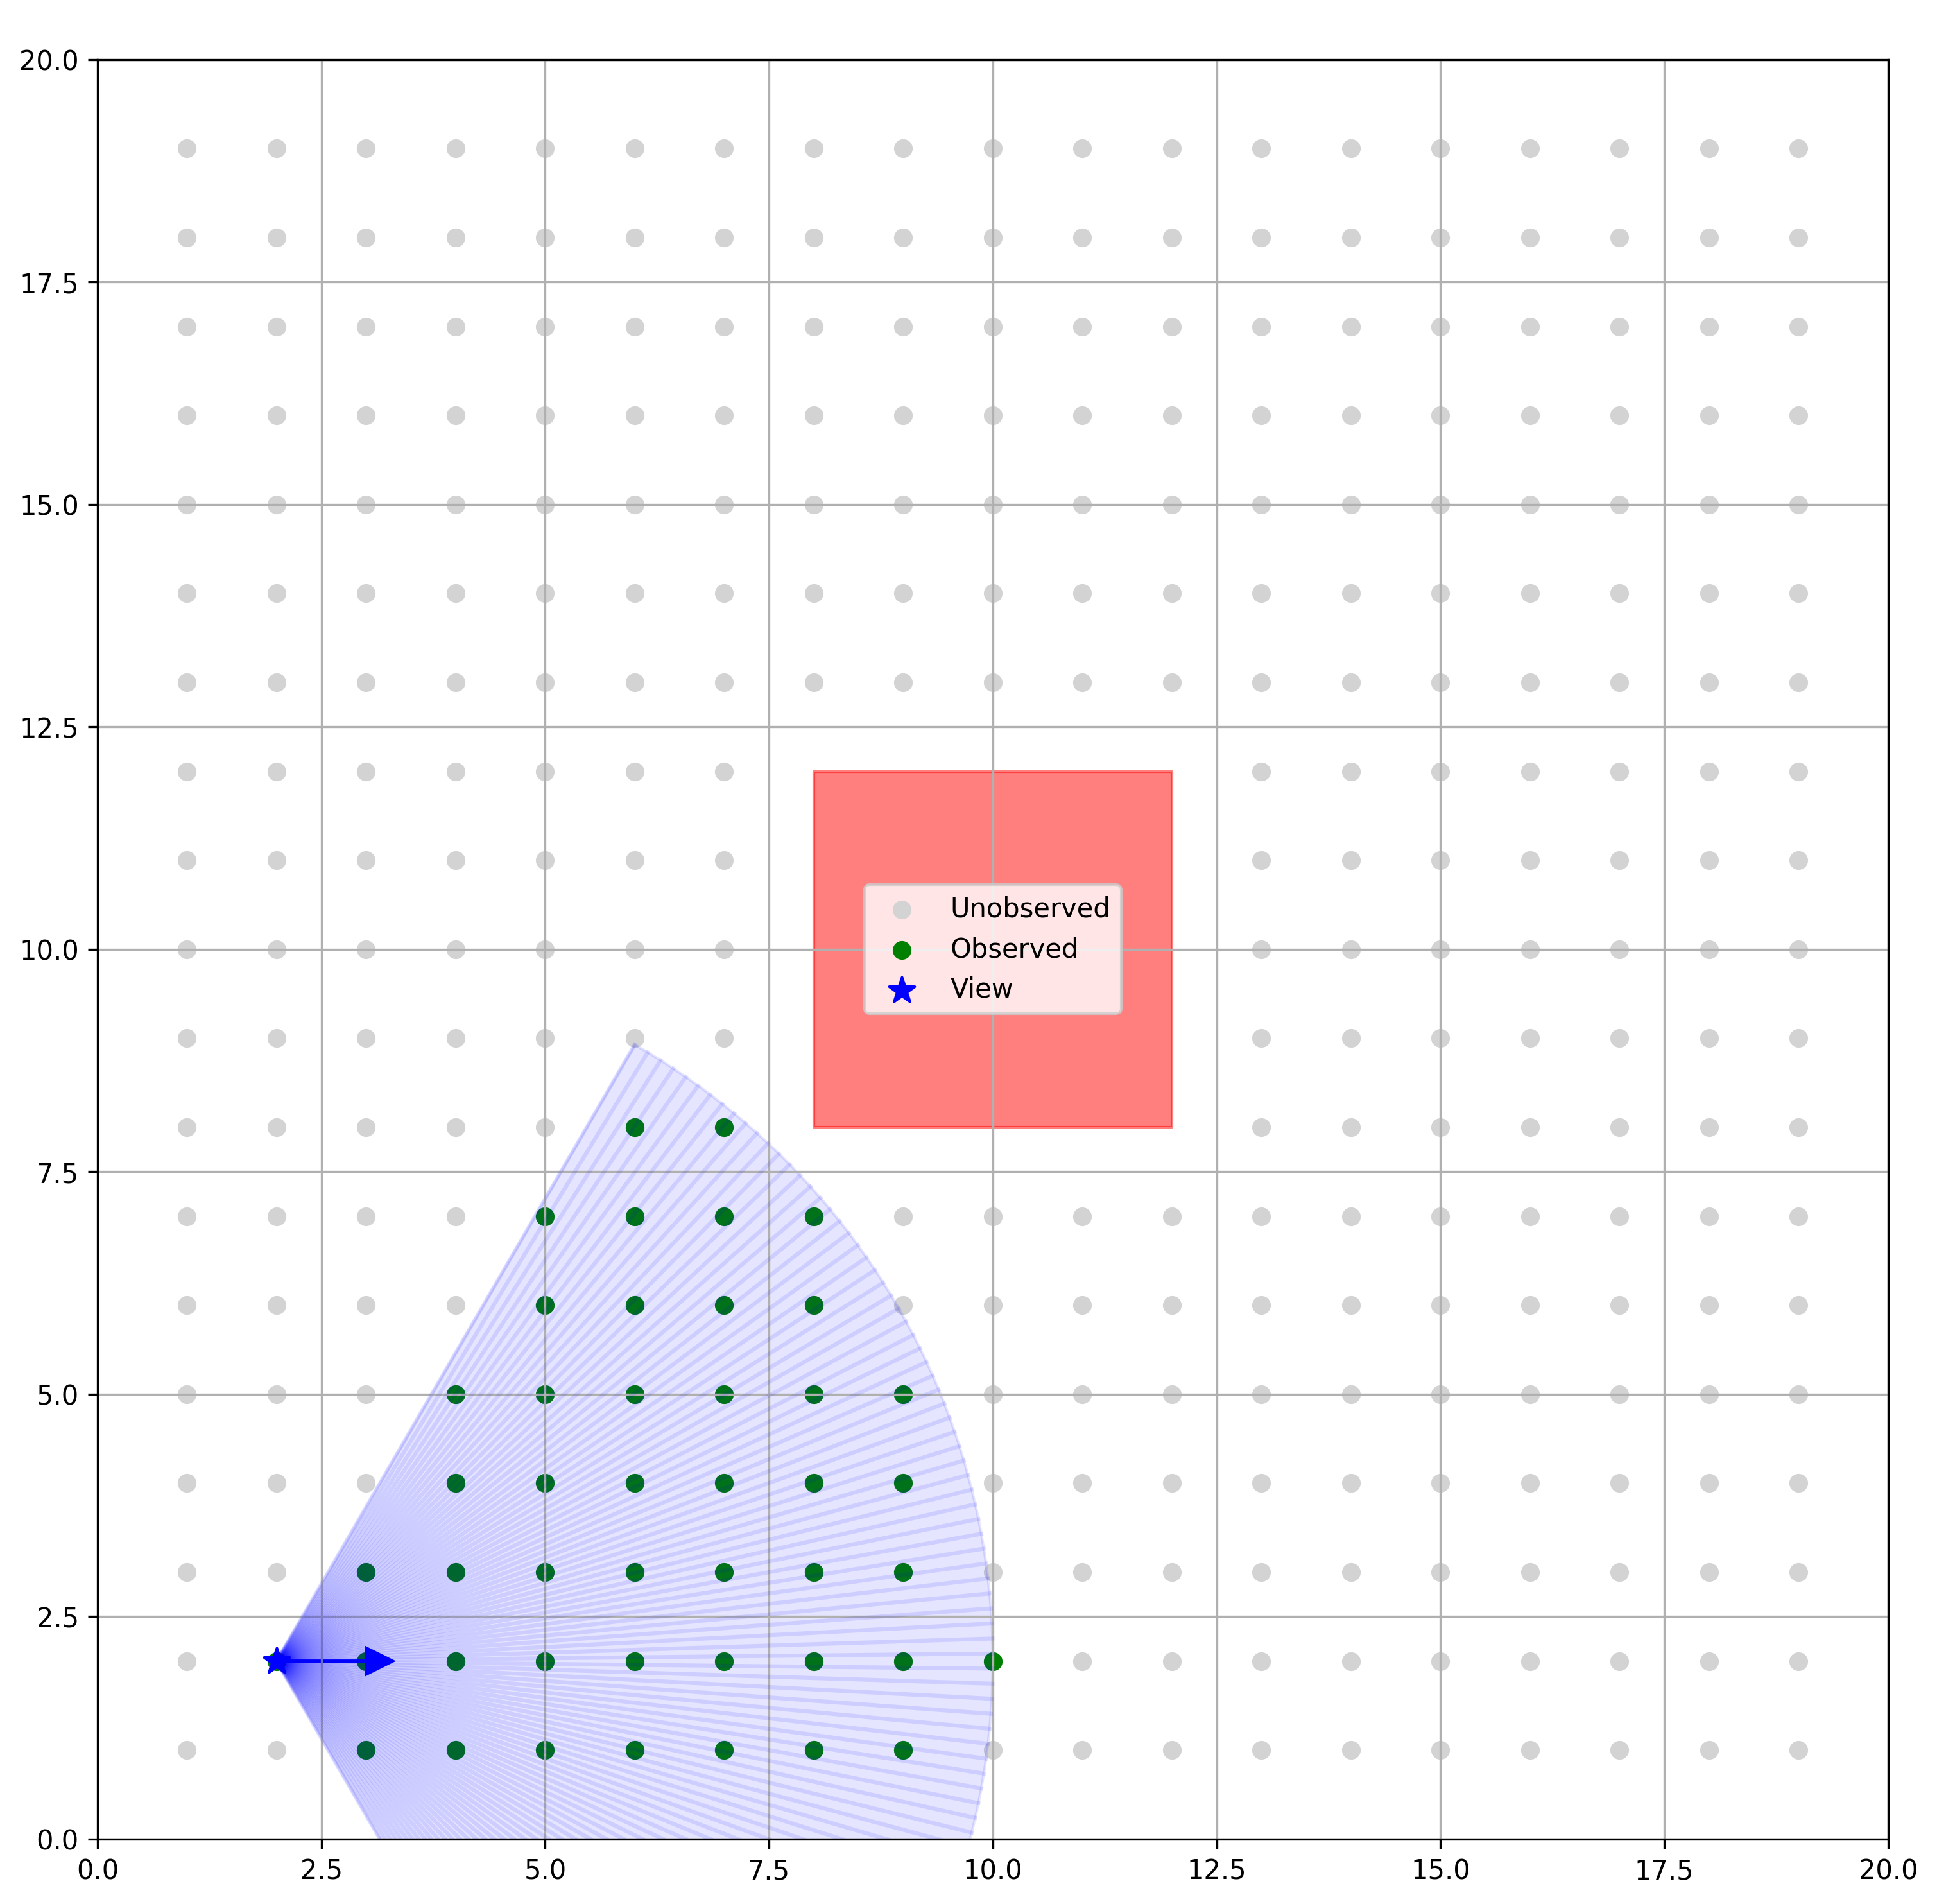}
    \caption{Scene 2: Central obstacle in area $20\times20$ $\text{unit}^2$.}
    \label{fig:s2}
\end{figure}
\begin{figure}
    \centering
    \includegraphics[width=0.8\linewidth]{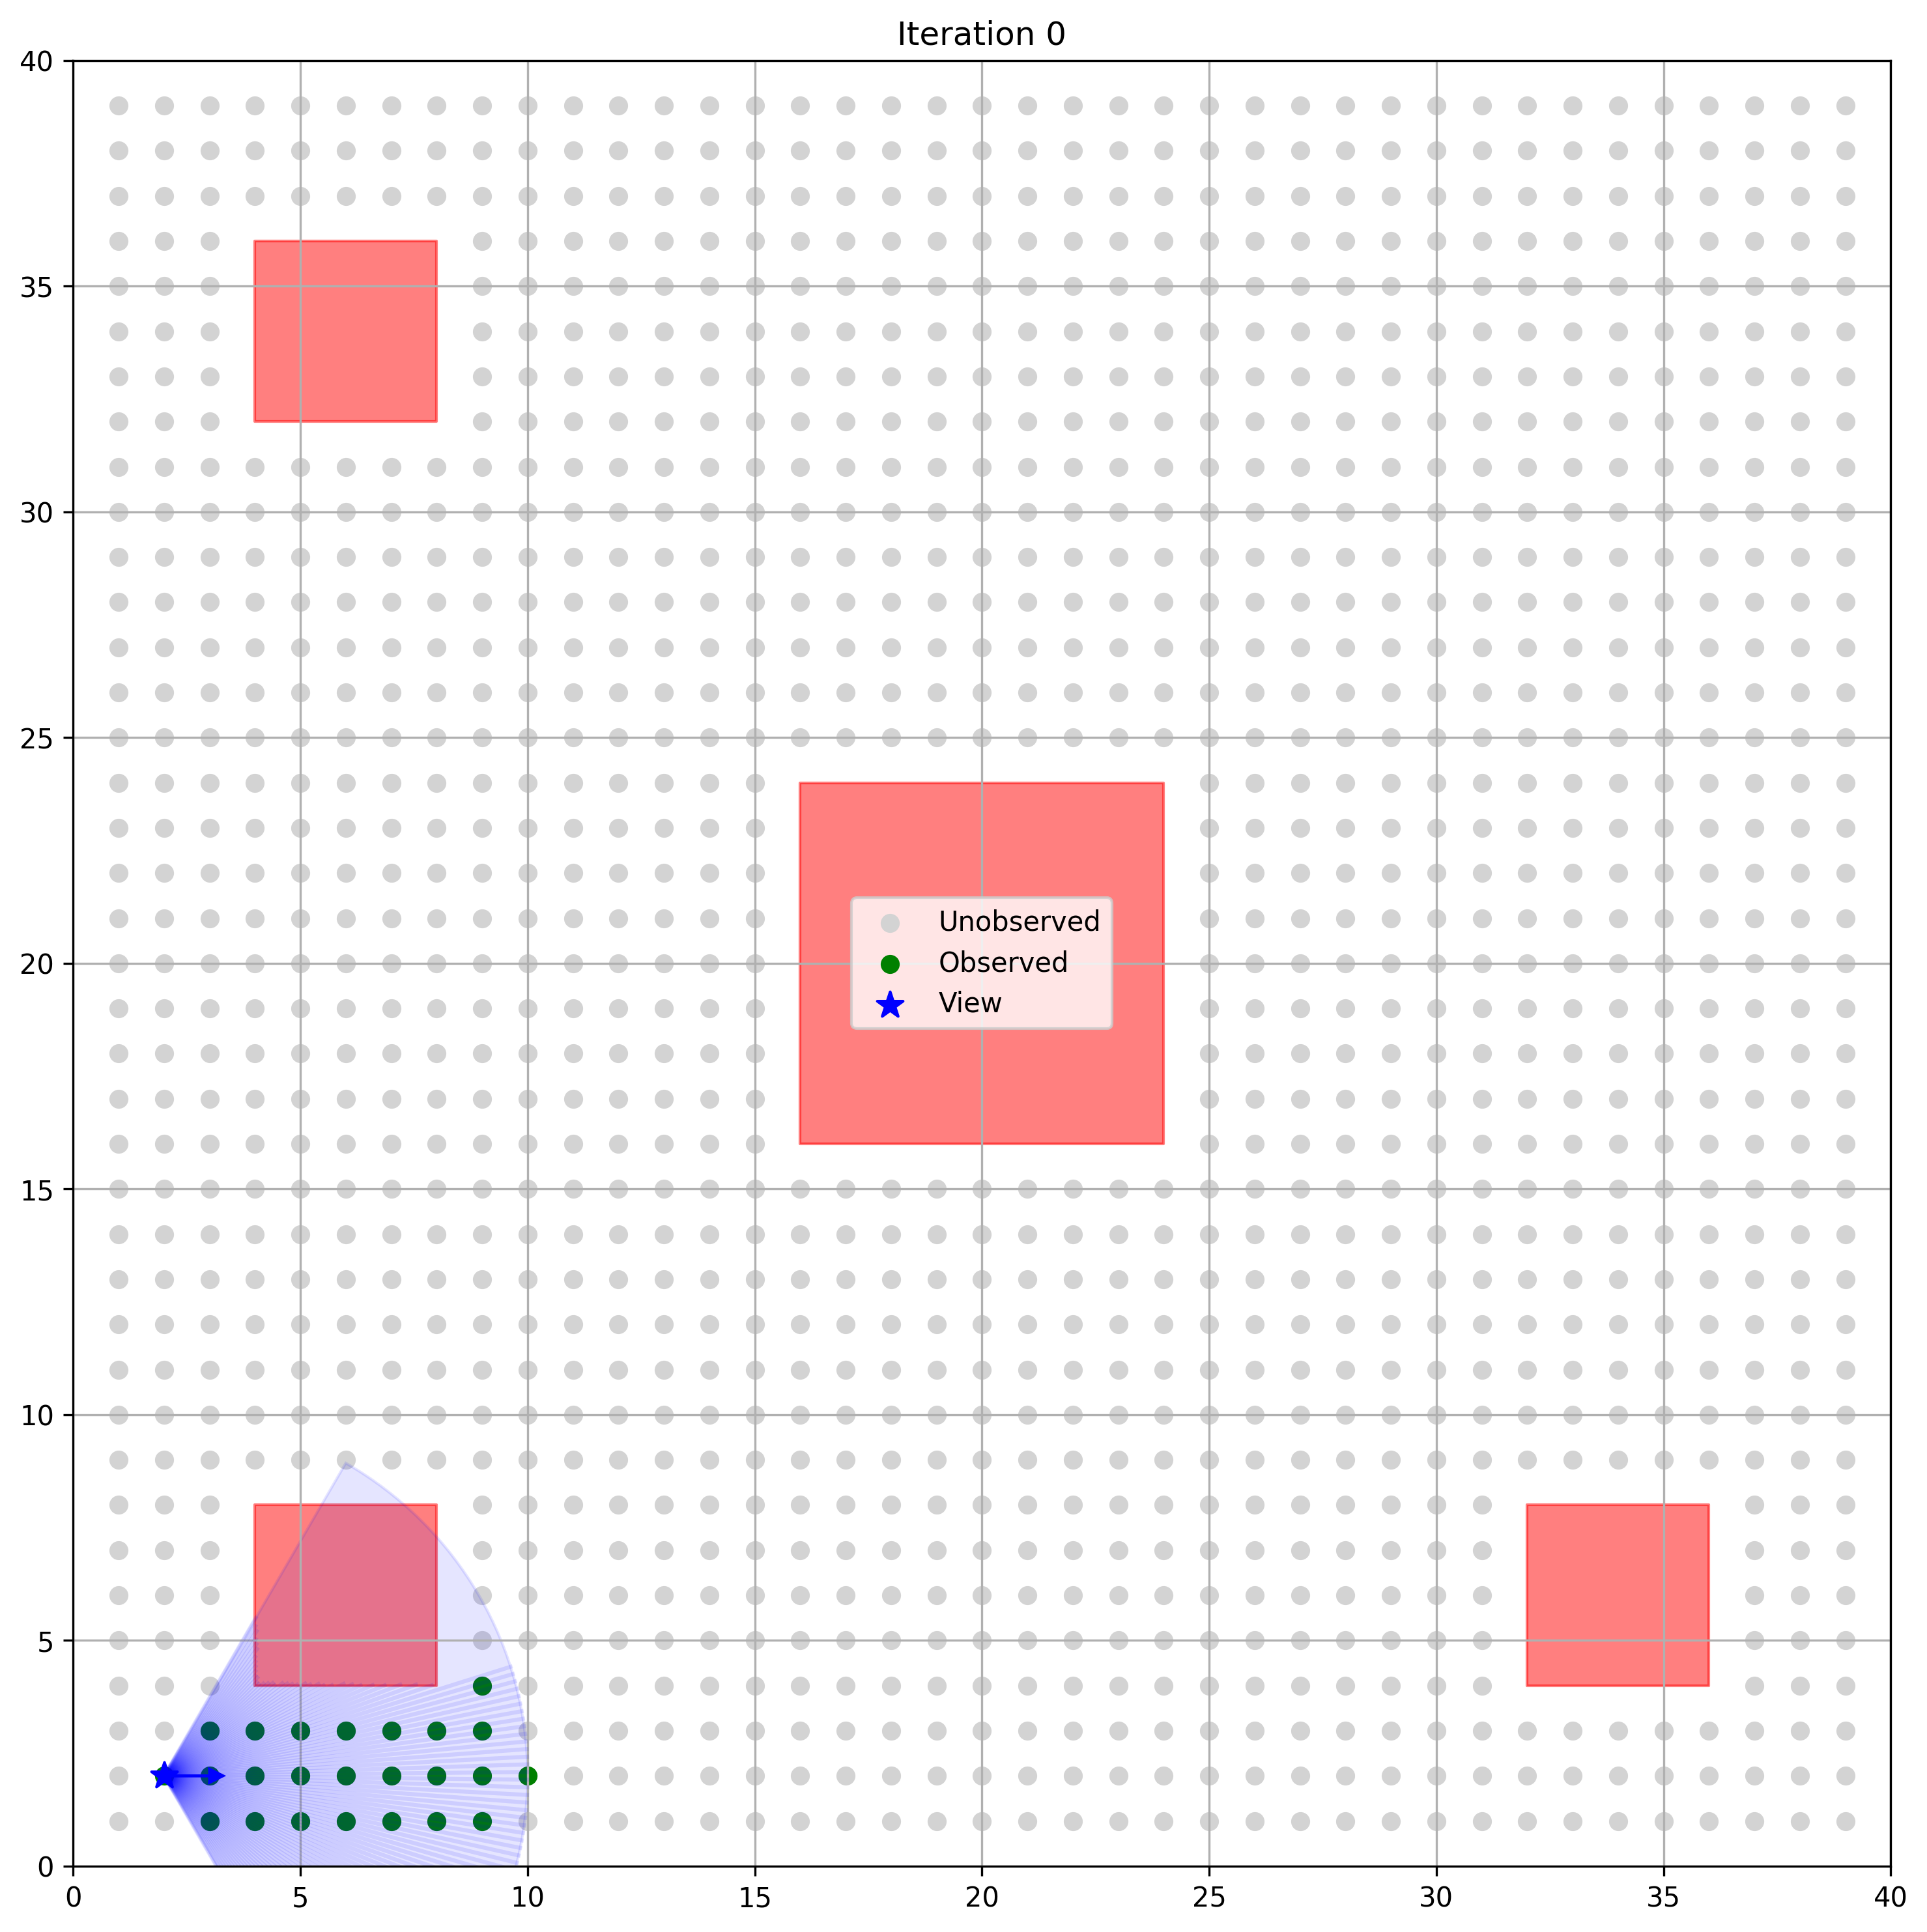}
    \caption{Scene 3: Surrounding and central obstacles in area $50\times50$ $\text{unit}^2$.}
    \label{fig:s3}
\end{figure}
The performance of our approach is evaluated by the coverage ratio, the normalized cost and state probability distribution evolution during the optimization process. Where the coverage ratio is simply defined as:
\begin{equation}
    \text{coverage ratio}=\frac{S_{observed}}{S}
\end{equation}
Where $S_{observed}$ denotes the observed area in the scene, and $S$ is the total area of the environment.

Normalized cost evaluates the overall cost evolution during the optimization process, which includes factors visibility to the unobserved area, movement cost, and regularization term.

the state probability distribution represents the likelihood of the quantum system being in each of the possible states, where each state corresponds to a unique combination of view parameters, including position and orientation. The probability distribution is derived from the quantum state $|\psi\rangle$ of the system, prepared by the variational ansatz. The probability of measuring a specific state $\textbf{x}$ is given by:
\begin{equation}
    P(\textbf{x})=|\langle\textbf{x}|\psi\rangle|^2
\end{equation}
As the optimization progresses, the distribution becomes more concentrated, with higher probabilities assigned to specific states, indicating that the algorithm is effectively narrowing down its search to the most advantageous solutions, thereby demonstrating the efficiency of the optimization process.

\section{Visualized Ansatz and Results}
\begin{figure*}
    \centering
    \includegraphics[width=1.0\linewidth]{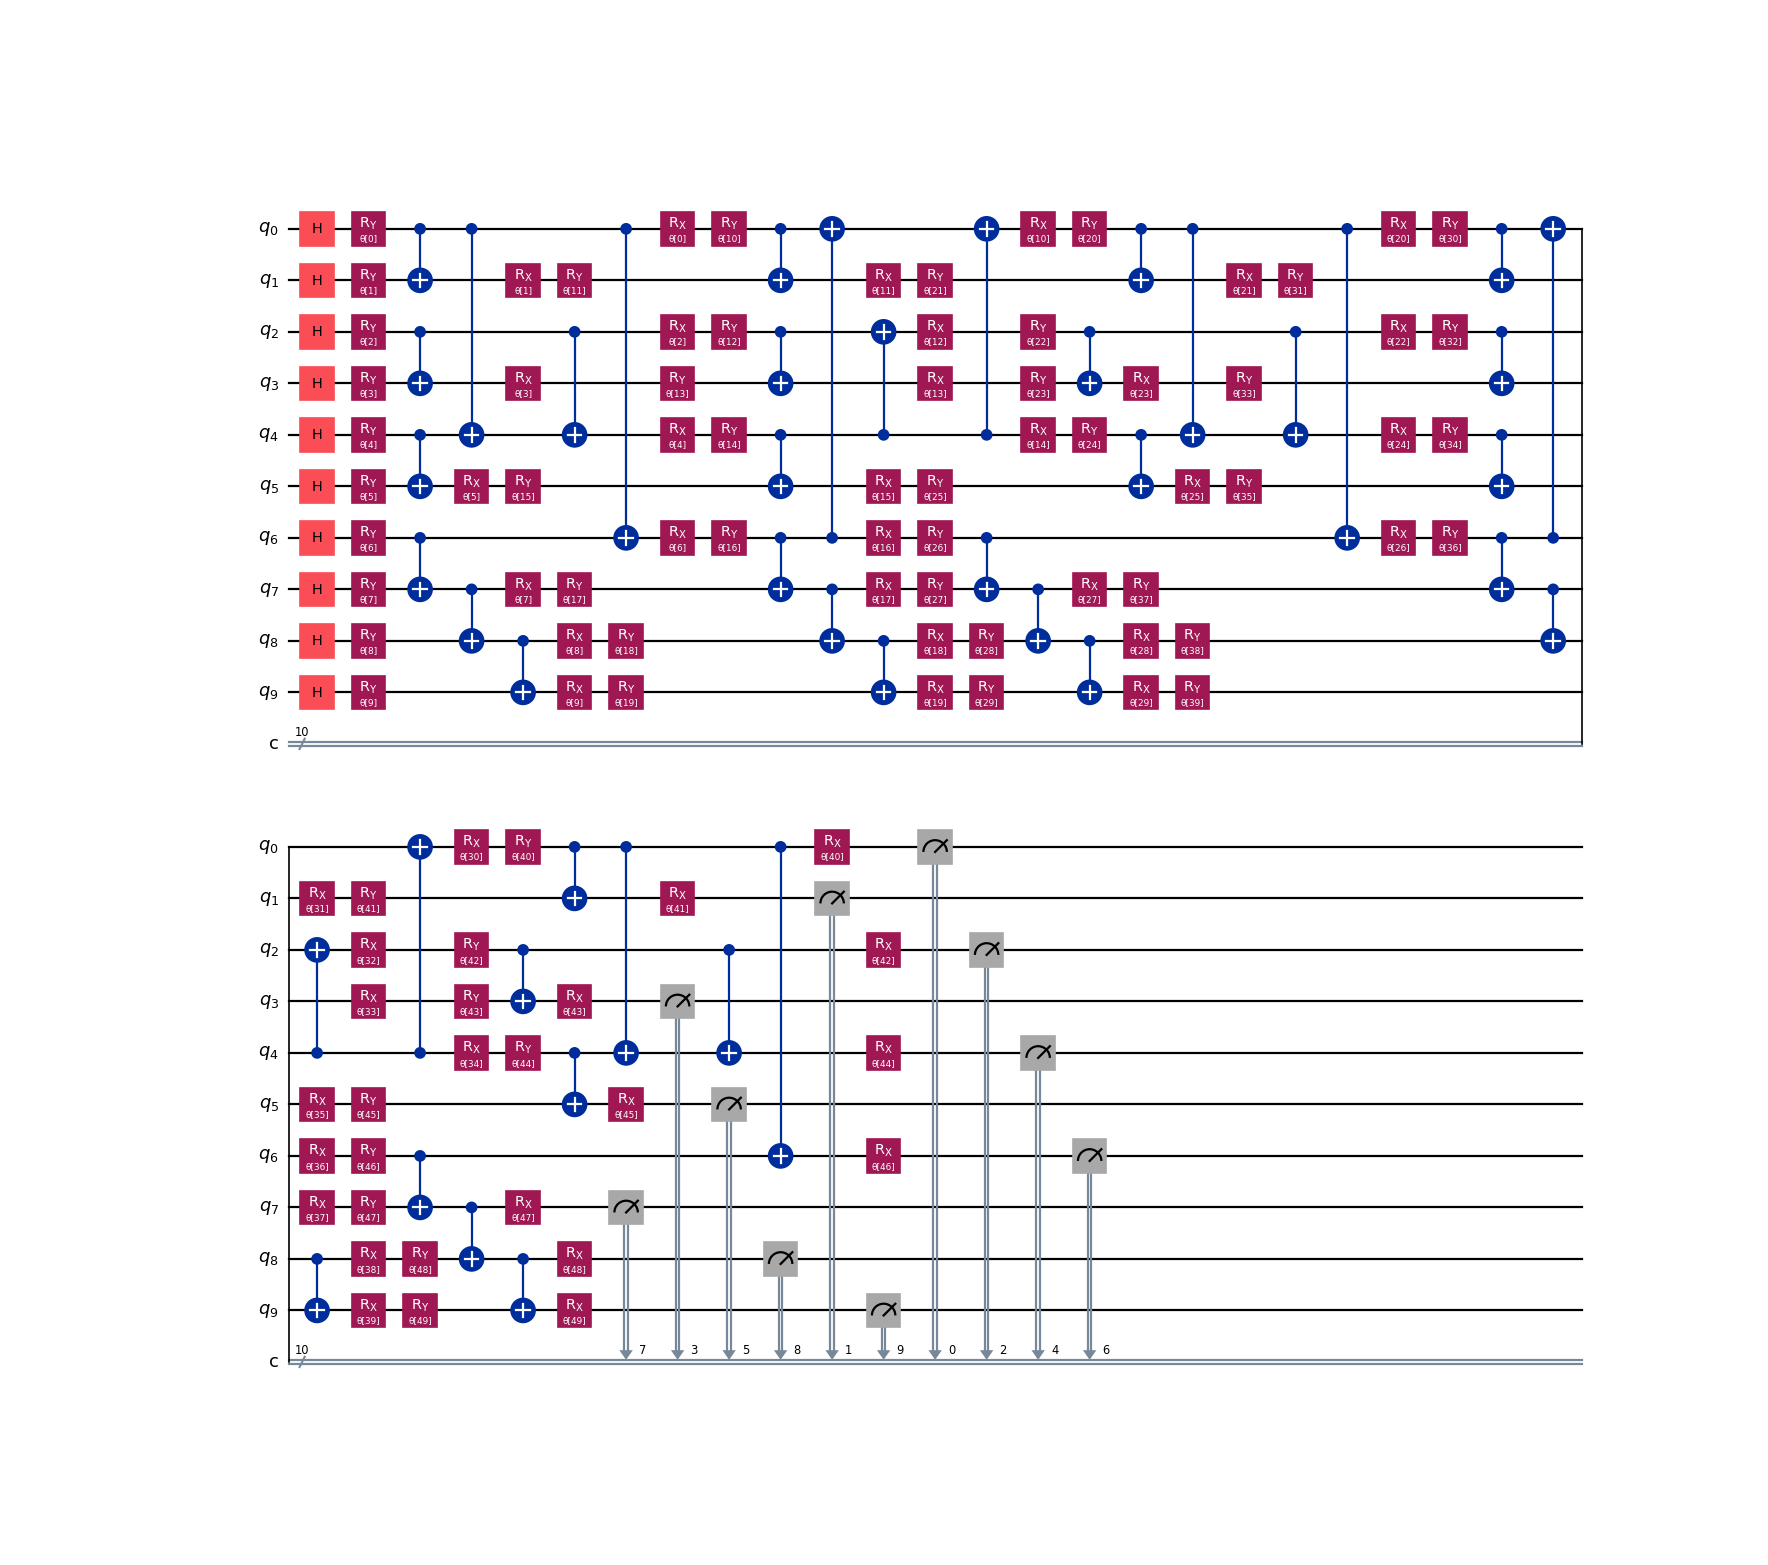}
    \caption{The full visualized circuit of our variational ansatz with $L=5$}
    \label{fig:full-circuit}
\end{figure*}
The full visualized ansatz is shown in Figure \ref{fig:full-circuit}. And a completed visualized experiment in Scene 2 is shown in Figure \ref{fig:visual_exp}.

\begin{figure*}
    \centering
    \includegraphics[width=1.0\linewidth]{}
    \caption{Full experiment in Scene 2}
    \label{fig:visual_exp}
\end{figure*}

\section{Classical Optimization Objective Function}

To effectively guide the quantum circuit parameter optimization, we define a comprehensive objective function that translates quantum measurements into viewpoint quality assessment. For parameters $\vec{\theta}$, the objective function is formulated as:

\begin{equation}
C(\vec{\theta}) = w_E C_E(\vec{\theta}) + w_M C_M(\vec{\theta}) + w_S C_S(\vec{\theta}) + w_R C_R(\vec{\theta})
\end{equation}

where:

\begin{itemize}
\item $C_E(\vec{\theta})$ represents the exploration cost, computed as the negative of expected information gain from a viewpoint decoded from parameters $\vec{\theta}$. This term favors viewpoints that maximize visibility of previously unobserved areas.

\item $C_M(\vec{\theta})$ represents the movement cost, proportional to the travel distance normalized by maximum observation distance: $C_M(\vec{\theta}) = \min(d_{\text{travel}}/d_{\text{max}}, 1.0)$.

\item $C_S(\vec{\theta})$ represents the safety cost, which penalizes viewpoints that are too close to obstacles: $C_S(\vec{\theta}) = 1.0 - 1.0/(1.0 + e^{-(d_{\text{obs}} - d_{\text{travel}})})$.

\item $C_R(\vec{\theta})$ represents a regularization cost that prevents excessive parameter changes between iterations, promoting smoother viewpoint transitions.
\end{itemize}

The weights $w_E$, $w_M$, $w_S$, and $w_R$ are adaptive, changing with exploration progress. Notably, $w_E = 1.0 + c$ (where $c$ is the coverage ratio) increases as exploration progresses, emphasizing information gain in later stages when unexplored regions become more difficult to locate.

To mitigate the effects of noisy quantum measurements, we employ an exponential moving average with factor $\alpha = 0.8$ to smooth cost components across iterations:

\begin{equation}
C_i^{(t)} = \alpha C_i^{(t-1)} + (1-\alpha)C_i^{(t)}
\end{equation}

This objective function guides the SPSA optimizer in finding optimal quantum circuit parameters that encode effective next viewpoints.

\section{Classical Fallback Strategy}

To ensure physical feasibility of the quantum-optimized solutions, we impose a hard constraint that projects quantum solutions onto the manifold of known free configurations. Formally, let $v_{q} = (x_q, y_q, \theta_q) \in \mathcal{C}$ be the viewpoint generated by quantum optimization, and let $\mathcal{F}_t \subset \mathcal{C}$ denote the known free configuration space at iteration $t$, defined as:

\begin{equation}
\mathcal{F}_t = \{v = (x, y, \theta) \in \mathcal{C} \mid \mathcal{M}_t(x, y) = 1\}
\end{equation}

where $\mathcal{M}_t(x, y) = 1$ indicates that position $(x, y)$ is observed and confirmed to be obstacle-free in the observation map at iteration $t$.

When $v_q \notin \mathcal{F}_t$, we apply a constrained projection operator $\mathcal{P}: \mathcal{C} \rightarrow \mathcal{F}_t$ that preserves directional intent while ensuring feasibility:

\begin{equation}
v_{t+1} = \mathcal{P}(v_q) = \arg\max_{v \in \mathcal{F}_t} \{\|v - v_t\|_2 \mid (v - v_t) \cdot (v_q - v_t) > 0\}
\end{equation}

subject to:
\begin{equation}
\theta_{t+1} = \theta_q
\end{equation}

This formulation identifies the furthest point along the ray from $v_t$ to $v_q$ that remains within the known free space $\mathcal{F}_t$, while preserving the orientation component $\theta_q$ from the quantum solution. The constraint $(v - v_t) \cdot (v_q - v_t) > 0$ ensures that the projected solution maintains the same directional intent as the original quantum solution.

This projection-based fallback strategy represents a hard constraint that guarantees physical feasibility while minimally perturbing the quantum-optimized exploration strategy, embodying the complementarity between quantum-derived global navigation policy and classical geometric constraint satisfaction.
